# Supplementary material for: The StarCraft Multi-Agent Challenges+ : Learning of Multi-Stage Tasks and Environmental Factors without Precise Reward Functions
Source: arXiv:2207.02007 source file (2022-07-07)
Supplement: Supplementary file 1 [file 2_Related_works.tex]

\section{Related works}
\label{sec:preliminaries}

Several reinforcement learning environments were designed to evaluate the ability to optimally execute multi-stage tasks to accomplish the desired goal. \cite{sohn2018subtask} introduced \textbf{Playground} which is a 2-dimensional environment characterized by a randomly generated multi-stage task graph that represents dependencies among multi-stage tasks. The goal of the agent is to find the optimal sequence of multi-stage tasks (for example, picking up a particular object) to maximize the reward. \textbf{FrankaKitchen} environment contains several household items and the task is to learn manipulating a 9 DoF robot arm to reach a particular state configuration. \cite{gupta2019subtask}. For example, the desired state requires the light on and the microwave open and each multi-stage task gives the sparse-reward. In contrast, SMAC+ scenarios only give rewards for the final objective (defeating enemies) and not to multi-stage tasks, hence the agents should implicitly learn to do multi-stage tasks.

Centralized Training \& Decentralized Execution (CTDE) is a widely adopted regime for MARL tasks \cite{oliehoek2008optimal}. The agents are trained with access to all global information. but act solely on local observations during execution. The CTDE research has been led by the development of environments.
\textbf{Multi-agent Particle Environment} provides a suite of 2-dimensional cooperative and competitive tasks where an agent interacts with other agents and landmarks. \cite{mordatch2018emergence} came up with the environment that allows for multi-agent's communication. Based on this framework, \cite{lowe2017multi, iqbal2019mpe} developed more general and challenging tasks. 
\cite{albrecht2015game} suggested \textbf{Level-Based Foraging} environment. Each agent is responsible for navigating the grid-world map and collecting items. This collection is successful only if the total level of all engaged agents levels is equal to or greater than the level of the item. 
\cite{xu2020learning} proposed a problem that requires sensor coordination in the two dimensional space in order to get ideal coverage while consuming low power, such as no missing targets or reducing redundant coverage. This environment regards action spaces as incrementally increasing or decreasing orientation of each sensor in 5 degrees.
Recently, \cite{papoudakis2021benchmarking} developed a \textbf{Multi-Robot Warehouse} environment in consideration of the sparse reward situation in MARL by rewarding agents for correctly completing a set of actions. Agents should identify and locate requested shelves to workstations on a grid-world warehouse.
\cite{peng2021facmac} developed \textbf{Multi-Agent MuJoCo}, allowing agents have cooperative and continuous robotic control. This environment assesses the ability of multiple agents inside a single robot to work together to complete a task. 

Most of the aforementioned environments are composed of simple tasks on limited state and action spaces. To incorporate more challenging factors such as partial observability and high-dimensional spaces, \cite{samvelyan2019starcraft} offered \textbf{SMAC}, an environment based on the Real-Time Strategy game StarCraft \uppercase\expandafter{\romannumeral2}. SMAC is used to assess micro-control of each agent to cooperatively eliminate opponents under unfavorable situations. Specifically, all scenarios in the SMAC are categorized into three levels of difficulties, referred to Easy, Hard, Super-Hard and such difficulties are determined by the number of allies units and its combination. Along the SMAC environment, \cite{papoudakis2021benchmarking} provided comprehensive benchmark results of 9 MARL algorithms total twenty-five tasks including 2-dimensional tasks and SMAC \cite{papoudakis2021benchmarking}. They illustrated that no algorithm outperforms all tasks; nevertheless policy gradient based MARL algorithms marginally have a high performance. However, since recent studies found that distributional value based algorithms consistently achieve high performance on the SMAC, this study does not reflect the current trend in research\cite{sun2021dfac, learning5disentangling}.

Although its challenging characteristics, there is no topographical change in SMAC except one scenario and only simple grounds are considered. Furthermore, as mentioned earlier, all scenarios considered only the cases against naturally approaching opponents. SMAC$^{+}$ introduces more complex scenarios where agents should learn to exploit environmental factors and implicit multi-stage tasks. Furthermore, we take a step to evaluate the abilities of MARL algorithms such as exploration strategies in the proposed SMAC$^{+}$ environment.
