# Supplementary material for: The StarCraft Multi-Agent Challenges+ : Learning of Multi-Stage Tasks and Environmental Factors without Precise Reward Functions
Source: arXiv:2207.02007 source file (2022-07-07)
Supplement: Supplementary file 2 [file 6_Case_study.tex]

\section{Case Study}

In this section, we  compare the learned policies with case studies of the results in \ref{sec:experiments}.

\paragraph{Defensive Scenario}
In the \texttt{super hard} in defense scenarios, enemies approach along with both left and right sides. \autoref{fig:def_shard} shows how algorithms are learned to utilize environmental factors. In case of MADDPG that records the best performance in this scenario, move two tanks to the left side and the remaining agents to the right side. As in \autoref{fig:def_shard}(a) and (b), this fully exploits environmental factors by placing units on the hill at the left side and units behind tree at the right side. On the other hand, DRIMA decides to move one tank to the left side and all other agents to the right side. The reason the win-rate of DRIMA is less than MADDPG is that beating all enemies on the left side by only one tank is not easy. When you see \autoref{fig:def_shard}(c) and (d), we identify that QMIX makes it worse. It move all agents forward the left side and then agents defeat some enemies and do not try to fight them in the other side.

\begin{figure}[t]{
    \begin{center}
        \subfigure[Left-side battle by MADDPG]{%
            \includegraphics[width=0.23\columnwidth]{Figures/4_Experiments/4_1_Defense/4_def_left_maddpg.png}
            \label{fig:def_maddpg_left}
        }
        \subfigure[Right-side battle by MADDPG]{%
            \includegraphics[width=0.23\columnwidth]{Figures/4_Experiments/4_1_Defense/4_def_right_maddpg.png}
            \label{fig:def_maddpg}
        }
        \subfigure[Left-side battle by QMIX]{%
            \includegraphics[width=0.23\columnwidth]{Figures/4_Experiments/4_1_Defense/4_def_left_qmix.png}
            \label{fig:def_qmix_left}
        }
        \subfigure[Right-side battle by QMIX]{%
            \includegraphics[width=0.23\columnwidth]{Figures/4_Experiments/4_1_Defense/4_def_right_qmix.png}
            \label{fig:def_qmix}
        }
    \end{center}
    }
    \caption{Defense super hard scenario replays with MADDPG, DRIMA, QMIX.}
    \label{fig:def_shard}
    \vskip -0.1in
\end{figure}
