# Supplementary material for: The StarCraft Multi-Agent Challenges+ : Learning of Multi-Stage Tasks and Environmental Factors without Precise Reward Functions
Source: arXiv:2207.02007 source file (2022-07-07)
Supplement: Supplementary file 3 [file Reward_engineering.tex]

\section{Reward Engineering}

\paragraph{Multi-stage task oriented reward} In offense scenarios, there is a clear multi-stage task that is finding enemies to fight. Since if agents didn't find any opponents, they can't get rewards from them. In offense hard scenario, QMIX does not show proper improvement in the winning rate with learning. It is because of the failure in searching. I which described in \autoref{overview}(a), In \autoref{fig:reward_engineering}(b), Although they go near enemies, they cannot climb the uphill. We want to solve this problem with simple reward engineering while expecting to give not only gain from fighting against opponents but also gain from distance from them. The alternative reward at time step $t$ before normalize is \autoref{eqn:reward_function}. We normalize this reward with the maximum alternative reward of the map. 
\begin{equation}
    \begin{aligned}
    \label{eqn:reward_function}
        R_{alt}^t = (\sum_{a}\sum_{e}d(a_{pos}^t, e_{pos}^t) - \sum_{a}\sum_{e}d(a_{pos}^{t-1}, e_{pos}^{t-1}))
    \end{aligned}
\end{equation}
where each $a$ and $e$ is agents and enemies, $d$ is euclidian distance and $pos$ means position. We test the alternative reward function in two ways. Using the alternative function until certain time steps like a step function, mixing it with basic reward function until the end, 2:8.

\begin{figure}[!h]{
    \begin{center}
        \subfigure[Comparing the alternative reward and basic reward]{
            \includegraphics[width=0.4\columnwidth]{Figures/A_5_Reward_engineering/qmix_reward_eng.png}
            \label{fig:basic_alt_compare}
        }
        \subfigure[QMIX with the basic reward at training step 10M]{
            \includegraphics[width=\columnwidth]{Figures/A_5_Reward_engineering/off_superhard_normal_reward_qmix.jpg}
            \label{fig:qmix_normal_reward}
        }
        \subfigure[QMIX with the alternative reward at training step 500k]{
            \includegraphics[width=\columnwidth]{Figures/A_5_Reward_engineering/off_superhard_reward_engineered_qmix.jpg}
            \label{fig:qmix_alt_reward}
        }
    \end{center}
    }
    \caption{(a) Performance comparison with basic and alternative reward function. (b),(c) Time ordered scene in replays in offense superhard. The sequences are captured at the same time. (c) is trained with the alternative reward function until 300k timestep.}
    \label{fig:reward_engineering}   
\end{figure}

\begin{figure}[!h]{
    \begin{center}
        \subfigure[QMIX with the basic reward at training step 10M]{
            \includegraphics[width=\columnwidth]{Figures/A_5_Reward_engineering/off_ultrahard_normal_qmix.jpg}
            \label{fig:qmix_normal_reward_uhard}
        }
        \subfigure[QMIX with the alternative reward at training step 800k]{
            \includegraphics[width=\columnwidth]{Figures/A_5_Reward_engineering/off_ultrahard_reward_qmix.jpg}
            \label{fig:qmix_alt_reward_uhard}
        }
    \end{center}
    }
    \caption{Time ordered scene in replays in offense ultrahard. The sequences are captured at the same time. (b) is trained with the alternative reward function until 800k timestep.}
    \label{fig:reward_engineering_uhard}   
\end{figure}

\paragraph{Result} \autoref{fig:reward_engineering}(a) shows drastic improved results. After applying alternative reward function for multi-stage task, QMIX agents directly head for the location where enemies at, as shown in \autoref{fig:reward_engineering} (c). This change makes QMIX appears to have completely solved the problem of multi-stage task. Even though agents don't fight a lot to approach enemies, they naturally fight with enemies to get closer to other enemies. 

However, in offense ultra hard scenario, the simple distance reward function doesn't work as in \autoref{fig:reward_engineering_uhard}. Although \autoref{fig:reward_engineering_uhard}(a) show QMIX could learn with basic reward function in ultra hard scenario. \autoref{fig:reward_engineering_uhard}(b) illustrate finding enemies with reward engineering is failed. It doesn't show any improvement, even it has worse performance.
